# Supplementary material for: In Situ Translational Hand-Eye Calibration of Laser Profile Sensors using Arbitrary Objects
Source: arXiv:2103.11981 source file (2021-03-22)
Supplement: Supplementary file 1 [file appendix.tex]

\appendices
\textcolor{red}{
\section{Demonstration of Theorem~{1}}
\label{appendix}
}
\textcolor{red}{
We analyze the rank of matrix $A$ for different values of $m$. For the sake of readability, in this demonstration we define ${}^B R_i := {}^B R_{E^i_1}$
}
\textcolor{red}{
\subsubsection{$m =1$}
As $A$ is a ${3m \times 6}$ matrix, it is not possible for it to be full column rank (i.e. $rank(A) = 6$) if $m = 1$, as we have that $A$ is a $3 \times 6$ matrix.
}

\textcolor{red}{
\subsubsection{$m = 2$}
For $m =2$ we have that the matrix A is:
\begin{equation*}
    A = \begin{bmatrix} 1_3 &  - {}^B R_{1} \\ 1_3 &  - {}^B R_{2} \end{bmatrix}.
\end{equation*}
Any matrix is not full column rank if its nullspace has size different from $0$, i.e. if it exists a vector $v = \begin{bmatrix} v_a \\ v_b \end{bmatrix} \in \mathbb{R}^6$ different from the zero vector for which:
\begin{equation*}
    Av = \begin{bmatrix} 1_3 &  - {}^B R_{1} \\ 1_3 &  - {}^B R_{2} \end{bmatrix} \begin{bmatrix} v_a \\ v_b \end{bmatrix} = 0_6 .
\end{equation*}
}
\textcolor{red}{
This equation is equivalent to the system of equations:
\begin{align*}
    v_a &= {}^B R_1 v_b, \\
    v_b &= {}^1 R_2 v_b. 
\end{align*} 
}
\textcolor{red}{
If we indicate as $a_{1,2} := axis({}^1 R_2) \in \mathbb{R}^3$ the rotation axis of the rotation matrix ${}^1 R_2$, we have that $a_{1,2} = {}^1 R_2 a_{1,2}$, so any non-zero vector of the form (where $k$ is any non-zero real number):
\begin{equation*}
    v = 
    \begin{bmatrix}
    k {}^B R_1 a_{1,2} \\
     a_{1,2}
    \end{bmatrix} ,
\end{equation*}
belongs to the nullspace of the matrix A, that means that A is not full-column rank for any value of ${}^B R_1$ and ${}^B R_2$.
}
\textcolor{red}{
\subsubsection{$m = 3$}
For $m =3$ we have that the matrix A is:
\begin{equation*}
    A = \begin{bmatrix} 1_3 &  - {}^B R_{1} \\
                        1_3 &  - {}^B R_{2} \\
                        1_3 &  - {}^B R_{3} \end{bmatrix} .
\end{equation*}
The nullspace of A is composed by the vectors $v = \begin{bmatrix} v_a \\ v_b \end{bmatrix} \in \mathbb{R}^6$ for which the following holds:
\begin{equation*}
    Av =  \begin{bmatrix} 1_3 &  - {}^B R_{1} \\
                        1_3 &  - {}^B R_{2} \\
                        1_3 &  - {}^B R_{3} \end{bmatrix}\begin{bmatrix} v_a \\ v_b \end{bmatrix} = 0_6  .
\end{equation*}
}
\textcolor{red}{
This equation is equivalent to the system of equations:
\begin{align*}
    v_a &= {}^B R_1 v_b, \\
    v_b &= {}^1 R_2 v_b, \\
    v_b &= {}^1 R_3 v_b.
\end{align*}
If we indicate as $a_{1,2} := axis({}^1 R_2) \in \mathbb{R}^3$ and $a_{1,3} := axis({}^1 R_3) \in \mathbb{R}^3$ the rotation axis of the rotation matrices ${}^1 R_2$ and ${}^1 R_3$, we have that for any non-zero solution of this equation, $v_b$ needs to be parallel to both $a_{1,3}$ and  $a_{2,3}$, and this is not possible  if $a_{1,3}$ and  $a_{2,3}$ are not parallel. From this, we can conclude that in the case $m=3$ if the rotation axis $a_{1,3}$ and  $a_{2,3}$ are not parallel, then the only element of the nullspace of A is the zero vector, and the matrix A is full-column rank.
}
